# Supplementary material for: Sign-reversal and non-monotonicity of chirality-related anomalous Hall effect in highly conductive metals
Source: arXiv:2502.04886 source file (2025-02-07)
Supplement: Supplementary file 1 [file suppl.pdf]

# Supplemental Material to
## "*Sign-reversal and non-monotonicity of chirality-related anomalous Hall effect in highly conductive metals*"

Ryunosuke Terasawa,[1] Masafumi Udagawa,[2] and Hiroaki Ishizuka[1]

[1]*Department of Physics, Institute of Science Tokyo, Meguro, Tokyo, 152-8551, Japan*

[2]*Department of Physics, Gakushuin University, Mejiro, Tossima-ku, Tokyo 171-8588, Japan*

(Dated: January 28, 2025)

## I. SECOND BORN APPROXIMATION

To study the AHE by skew scattering, we compute the asymmetric terms in the scattering rate using the second Born approximation. Within this approximation, the symmetric $w^{+}_{\boldsymbol{k}\mu\to\boldsymbol{k}'\nu}$ and asymmetric $w^{-}_{\boldsymbol{k}\mu\to\boldsymbol{k}'\nu}$ parts of the scattering rate read

$$
\begin{aligned}
w^{+}_{\boldsymbol{k}\mu\to\boldsymbol{k}'\nu} =& 2\pi \left| \langle \boldsymbol{k}'\nu \,|\, H_K \,|\, \boldsymbol{k}\mu \rangle \right|^2 \delta(\epsilon_{\boldsymbol{k}\mu} - \epsilon_{\boldsymbol{k}'\nu}) \\
&+ 4\pi \sum_{\boldsymbol{p},\lambda} \left[ \langle \boldsymbol{k}'\nu \,|\, H_K \,|\, \boldsymbol{k}\mu \rangle \langle \boldsymbol{k}\mu \,|\, H_K \,|\, \boldsymbol{p}\lambda \rangle \langle \boldsymbol{p}\lambda \,|\, H_K \,|\, \boldsymbol{k}'\nu \rangle \right] \frac{\mathcal{P}}{\epsilon_{\boldsymbol{k}\mu} - \epsilon_{\boldsymbol{p}\lambda}} \delta(\epsilon_{\boldsymbol{k}\mu} - \epsilon_{\boldsymbol{k}'\nu}) \qquad \text{(S1)}
\end{aligned}
$$

$$
w^{-}_{\boldsymbol{k}\mu\to\boldsymbol{k}'\nu} = (2\pi)^2 \sum_{\boldsymbol{p},\lambda} \Im \left[ \langle \boldsymbol{k}'\nu \,|\, H_K \,|\, \boldsymbol{k}\mu \rangle \langle \boldsymbol{k}\mu \,|\, H_K \,|\, \boldsymbol{p}\lambda \rangle \langle \boldsymbol{p}\lambda \,|\, H_K \,|\, \boldsymbol{k}'\nu \rangle \right] \delta(\epsilon_{\boldsymbol{k}\mu} - \epsilon_{\boldsymbol{k}'\nu}) \delta(\epsilon_{\boldsymbol{k}\mu} - \epsilon_{\boldsymbol{p}\lambda}). \qquad \text{(S2)}
$$

For the quadratic Hamiltonian, the asymmetric part is

$$
w^{-}_{\boldsymbol{k}\mu\to\boldsymbol{k}'\nu} = \frac{2\pi J_K^3}{L^4} \sum_{i,j,l} \frac{k J_0(kR_{lj})}{v_k} \Im \left[ (\boldsymbol{S}_i \cdot \boldsymbol{\sigma})_{\mu\nu} \left( \boldsymbol{S}_j \cdot \boldsymbol{S}_l \sigma_0 + i \boldsymbol{\sigma} \cdot \boldsymbol{S}_j \times \boldsymbol{S}_l \right)_{\nu\mu} \exp\{-i\boldsymbol{k} \cdot \boldsymbol{R}_{li} + i\boldsymbol{k}' \cdot \boldsymbol{R}_{ji}\} \right] \delta(\varepsilon_{\boldsymbol{k}\mu} - \varepsilon_{\boldsymbol{k}'\nu}), \qquad \text{(S3)}
$$

$$
\begin{aligned}
=& \frac{2\pi J_K^3}{L^4} \sum_{i,j,l,n,m} \frac{k J_0(kR_{lj}) J_n(kR_{li}) J_m(kR_{ji})}{v_k} \\
&\times \mathrm{Im} \left[ (-i)^n i^m (\boldsymbol{S}_i \cdot \boldsymbol{\sigma})_{\mu\nu} \left( \boldsymbol{S}_j \cdot \boldsymbol{S}_l \sigma_0 + i \boldsymbol{\sigma} \cdot \boldsymbol{S}_j \times \boldsymbol{S}_l \right)_{\nu\mu} \exp\{in(\phi - \phi_{li})\} \exp\{im(\phi' - \phi_{ji})\} \right] \delta(\varepsilon_{\boldsymbol{k}\mu} - \varepsilon_{\boldsymbol{k}'\nu}), \qquad \text{(S4)}
\end{aligned}
$$

where $J_n(x)$ are the Bessel functions of the first kind, $v_k = k/m$, $\phi$ ($\phi'$) is the azimuth of $\boldsymbol{k}(\boldsymbol{k}')$, $\boldsymbol{k} = k(\cos(\phi), \sin(\phi))$, and $\phi_{li}$ is the azimuth of $\boldsymbol{R}_{li}$, $\boldsymbol{R}_{li} = R_{li}(\cos(\phi_{li}), \sin(\phi_{li}))$. Taking the average over the incident wave direction, the asymmetric part of the scattering rate becomes

$$
\begin{aligned}
w^{-}_{\boldsymbol{k}\mu\to\boldsymbol{k}'\nu} =& \frac{2\pi J_K^3}{L^4} \sum_{i,j,l,n} \frac{k J_0(kR_{lj}) J_n(kR_{li}) J_n(kR_{ji})}{v_k} \cos\{n(\phi_{ji} - \phi_{li} - \delta\phi)\} \\
&\times \mathrm{Im} \left[ (\boldsymbol{S}_i \cdot \boldsymbol{\sigma})_{\mu\nu} \left( \boldsymbol{S}_j \cdot \boldsymbol{S}_l \sigma_0 + i \boldsymbol{\sigma} \cdot \boldsymbol{S}_j \times \boldsymbol{S}_l \right)_{\nu\mu} \right] \delta(\varepsilon_{\boldsymbol{k}\mu} - \varepsilon_{\boldsymbol{k}'\nu}), \qquad \text{(S5)}
\end{aligned}
$$

where $\delta\phi = \phi' - \phi$. In this work, we focus on the $\sin(\delta\phi)$ term,

$$
\begin{aligned}
w^{-}_{\boldsymbol{k}\mu\to\boldsymbol{k}'\nu} =& \frac{4m\pi J_K^3}{L^4} \sum_{i,j,l} J_0(kR_{lj}) J_1(kR_{li}) J_1(kR_{ji}) (\hat{z} \cdot \hat{R}_{li} \times \hat{R}_{ji}) (\hat{z} \cdot \hat{k} \times \hat{k}') \\
&\times \left[ S_i^z (\boldsymbol{S}_j \times \boldsymbol{S}_l)^z \delta_{\mu\nu} + \left( S_i^x (\boldsymbol{S}_j \times \boldsymbol{S}_l)^x + S_i^y (\boldsymbol{S}_j \times \boldsymbol{S}_l)^y \right) \delta_{\bar{\mu}\nu} \right] \delta(\varepsilon_{\boldsymbol{k}\mu} - \varepsilon_{\boldsymbol{k}'\nu}). \qquad \text{(S6)}
\end{aligned}
$$

The Hall conductivity was calculated by combining Eq. (S6) and the Boltzmann equation.

## II. HALL CONDUCTIVITY FORMULAS FOR KAGOMÉ ICE

In this section, we show the formula for each contribution to the Hall conductivity $\sigma_a(a=A,\cdots,E)$, classified by the scattering process. Using $\sum_h \frac{2}{\sqrt{3}}a^2 = L^2$, $\sigma_a$ reads

$$\sigma_A = -\frac{4\sigma_0 k_F^2}{\sqrt{3}a^2}\chi_A J_0(k_F a)J_1(k_F a)^2, \tag{S7}$$

$$\sigma_B = \frac{4\sigma_0 k_F^2}{\sqrt{3}a^2}\chi_B \left[J_0(\sqrt{3}k_F a)J_1(k_F a)^2 + \frac{2}{\sqrt{3}}J_0(k_F a)J_1(\sqrt{3}k_F a)J_1(k_F a)\right], \tag{S8}$$

$$\sigma_C = -\frac{8\sigma_0 k_F^2 \chi_C}{\sqrt{3}a^2}\left[\frac{1}{\sqrt{3}}J_0(\sqrt{7}k_F a)J_1(\sqrt{3}k_F a)J_1(k_F a) + \frac{1}{\sqrt{7}}J_0(\sqrt{3}k_F a)J_1(\sqrt{7}k_F a)J_1(k_F a) + \frac{1}{\sqrt{21}}J_0(k_F a)J_1(\sqrt{3}k_F a)J_1(\sqrt{7}k_F a)\right], \tag{S9}$$

$$\sigma_D = -\frac{4\sigma_0 k_F^2}{\sqrt{3}a^2}\chi_D J_0(\sqrt{3}k_F a)J_1(\sqrt{3}k_F a)^2, \tag{S10}$$

$$\sigma_E = \frac{4\sigma_0 k_F^2}{\sqrt{3}a^2}\chi_E \left[J_0(3k_F a)J_1(\sqrt{3}k_F a)^2 + \frac{2}{\sqrt{3}}J_0(\sqrt{3}k_F a)J_1(\sqrt{3}k_F a)J_1(3k_F a)\right]. \tag{S11}$$

The contribution of each term to the AHE depends on its coefficient, the Bessel function, and which contribution dominates varies with the Fermi wavenumber. When $x \ll 1$, since the Bessel function is $J_0(x) \sim 1 - \frac{x^2}{4} + \frac{x^4}{64}$, $J_1(x) \sim \frac{x}{2} - \frac{x^3}{16}$ when $x$ is sufficiently small, the Hall conductivity can be approximated for small $k_F a$ as follows,

$$\sigma_A \sim \frac{\sigma_0 k_F^4}{\sqrt{3}}\chi_A \left[-1 + \frac{(k_F a)^2}{2} - \frac{5(k_F a)^4}{48}\right], \tag{S12}$$

$$\sigma_B \sim \frac{\sigma_0 k_F^4}{\sqrt{3}}\chi_B \left[3 - \frac{5(k_F a)^2}{2} + \frac{5(k_F a)^4}{6}\right], \tag{S13}$$

$$\sigma_C \sim \frac{\sigma_0 k_F^4}{\sqrt{3}}\chi_C \left[6 - 11(k_F a)^2 - \frac{49(k_F a)^4}{12}\right], \tag{S14}$$

$$\sigma_D \sim -\frac{3\sigma_0 k_F^4}{\sqrt{3}}\chi_D \left[1 - \frac{3(k_F a)^2}{2} + \frac{15(k_F a)^4}{16}\right], \tag{S15}$$

$$\sigma_E \sim \frac{9\sigma_0 k_F^4}{\sqrt{3}}\chi_E \left[1 - \frac{5(k_F a)^2}{2} + \frac{5(k_F a)^4}{2}\right]. \tag{S16}$$

Also, when $x \gg 1$, since the Bessel function is $J_0(x) \sim \sqrt{\frac{2}{\pi x}}\cos(x - \frac{\pi}{4})$, $J_1(x) \sim \sqrt{\frac{2}{\pi x}}\cos(x - \frac{3\pi}{4})$ when $x$ is sufficiently large, the Hall conductivity can be approximated for large $k_F a$ as follows,

$$\sigma_A \sim -\sqrt{\frac{2k_F}{3\pi a}}\frac{8\sigma_0}{\pi a^3}\chi_A \cos(k_F a - \frac{\pi}{4})\cos^2(k_F a - \frac{3\pi}{4}), \tag{S17}$$

$$\sigma_B \sim \sqrt{\frac{2k_F}{3\pi a}}\frac{8}{3^{\frac{1}{4}}\pi a^3}\chi_B \cos(k_F a - \frac{3\pi}{4})\left[\cos(\sqrt{3}k_F a - \frac{\pi}{4})\cos(k_F a - \frac{3\pi}{4}) + \frac{2}{\sqrt{3}}\cos(k_F a - \frac{\pi}{4})\cos(\sqrt{3}k_F a - \frac{3\pi}{4})\right], \tag{S18}$$

$$\sigma_C \sim -\sqrt{\frac{2k_F}{3\pi a}}\frac{16}{21^{\frac{1}{4}}\pi a^3}\chi_C \left[\frac{1}{\sqrt{3}}\cos(\sqrt{7}k_F a - \frac{\pi}{4})\cos(\sqrt{3}k_F a - \frac{3\pi}{4})\cos(k_F a - \frac{3\pi}{4}) + \frac{1}{\sqrt{7}}\cos(\sqrt{3}k_F a - \frac{\pi}{4})\cos(\sqrt{7}k_F a - \frac{3\pi}{4})\cos(k_F a - \frac{3\pi}{4}) + \frac{1}{\sqrt{21}}\cos(k_F a - \frac{\pi}{4})\cos(\sqrt{7}k_F a - \frac{3\pi}{4})\cos(\sqrt{3}k_F a - \frac{3\pi}{4})\right], \tag{S19}$$

$$\sigma_D \sim -\sqrt{\frac{2k_F}{3\pi a}}\frac{8\sigma_0}{3^{\frac{3}{4}}\pi a^3}\chi_D \cos(\sqrt{3}k_F a - \frac{\pi}{4})\cos^2(\sqrt{3}k_F a - \frac{3\pi}{4}), \tag{S20}$$

$$\sigma_E \sim \sqrt{\frac{2k_F}{3\pi a}}\frac{8\sigma_0}{3\pi a^3}\chi_E \left[\cos(3k_F a - \frac{\pi}{4})\cos^2(\sqrt{3}k_F a - \frac{3\pi}{4}) + \frac{2}{\sqrt{3}}\cos(\sqrt{3}k_F a - \frac{\pi}{4})\cos(\sqrt{3}k_F a - \frac{3\pi}{4})\cos(3k_F a - \frac{3\pi}{4})\right]. \tag{S21}$$

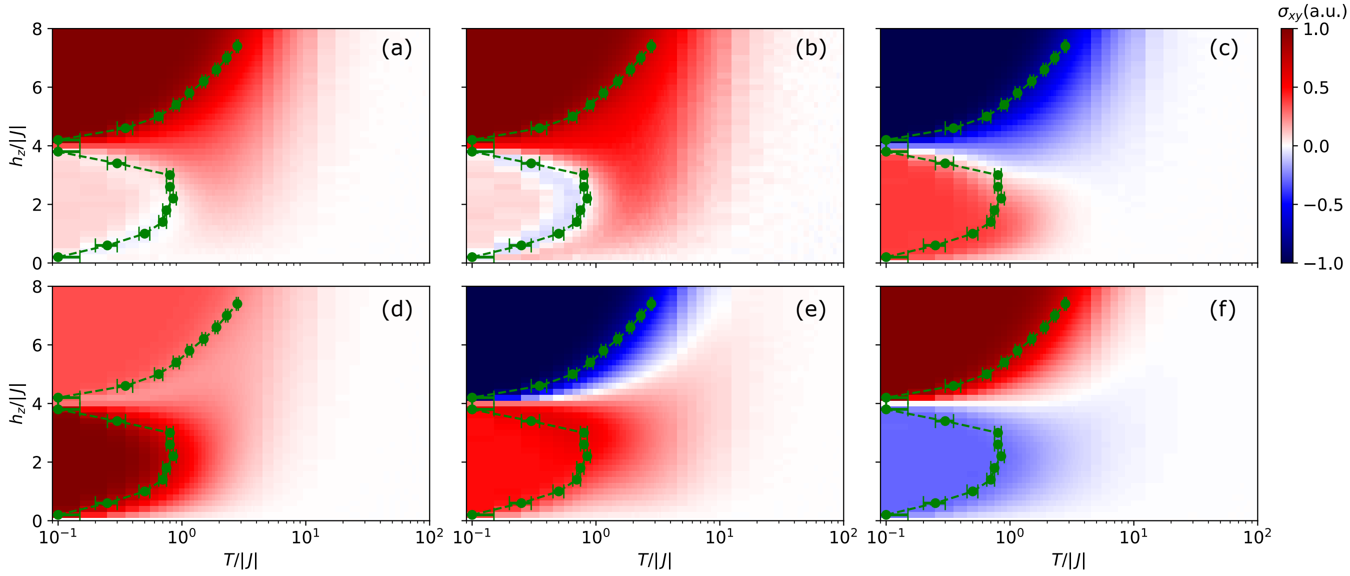


FIG. S1. Magnetic phase diagram of kagomé ice model and the contour plot of the anomalous Hall conductivity at (a) $k_F a = 0.1$, (b) $k_F a = 0.5$, (c) $k_F a = 1.0$, (d) $k_F a = 1.5$, (e) $k_F a = 2.5$, (f) $k_F a = 3.0$. The green dots represent the peak of specific heat.

The Hall conductivity shown in the main text was calculated using these equations.

## III. HALL CONDUCTIVITY

As discussed in the main text, the Hall conductivity $\sigma_{xy}$ for a given magnetic state exhibits a complex dependence on the Fermi wavenumber $k_F a$. Consequently, $\sigma_{xy}$ shows rich temperature and magnetic field dependencies as shown in Fig. S1. The contour plot similar to Fig. S1(a) appears at Fermi wavenumbers $k_F a \lesssim 0.4$; similarly, we find the temperature and magnetic field dependence similar to each figure in Fig. S1 at (b) $0.4 \lesssim k_F a \lesssim 0.7$, (c) $0.7 \lesssim k_F a \lesssim 1.2$, (d) $1.2 \lesssim k_F a \lesssim 1.6$, (e) $1.6 \lesssim k_F a \lesssim 2.5$, (f) $2.5 \lesssim k_F a \lesssim 3.0$.

## IV. HIGH-TEMPERATURE EXPANSION

In this section, we show the method to calculate the three spin correlations from the free energy. For the effective Ising model on kagomé lattice,

$$H_S = -\sum_{\langle i,j\rangle} J_{ij}\tau_i\tau_j - \sum_i h_i^z \tau_i, \tag{S22}$$

the free energy reads

$$F = -T\ln\left[\sum_{\{\tau_i\}=\pm 1} \mathrm{e}^{\sum_i \beta h_i^z \tau_i + \sum_{\langle i,j\rangle} \beta J_{ij}\tau_i\tau_j}\right]. \tag{S23}$$

By differentiating this, the average value of spin can be calculated as follows,

$$-\partial_{h_i^z} F = \frac{1}{Z} \sum_{\{\tau_i\}=\pm 1} \tau_i \mathrm{e}^{\sum_i \beta h_i^z \tau_i + \sum_{\langle i,j\rangle} \beta J_{ij}\tau_i\tau_j} = \langle \tau_i \rangle, \tag{S24}$$

$$\begin{aligned}
-T\partial_{h_i^z}\partial_{h_j^z} F =& \frac{1}{Z} \sum_{\{\tau_i\}=\pm 1} \tau_i\tau_j \mathrm{e}^{\sum_i \beta h_i^z \tau_i + \sum_{\langle i,j\rangle} \beta J_{ij}\tau_i\tau_j} \\
& - \frac{1}{Z^2} \sum_{\{\tau_i\}=\pm 1} \tau_i \mathrm{e}^{\sum_i \beta h_i^z \tau_i + \sum_{\langle i,j\rangle} \beta J_{ij}\tau_i\tau_j} \sum_{\{\tau_i\}=\pm 1} \tau_j \mathrm{e}^{\sum_i \beta h_i^z \tau_i + \sum_{\langle i,j\rangle} \beta J_{ij}\tau_i\tau_j} \\
=& \langle \tau_i\tau_j \rangle - \langle \tau_i \rangle\langle \tau_j \rangle,
\end{aligned} \tag{S25}$$

$$\begin{aligned}
-T^2\partial_{h_i^z}\partial_{h_j^z}\partial_{h_k^z} F =& \frac{1}{Z} \sum_{\{\tau_i\}=\pm 1} \tau_i\tau_j\tau_k \mathrm{e}^{\sum_i \beta h_i^z \tau_i + \sum_{\langle i,j\rangle} \beta J_{ij}\tau_i\tau_j} \\
& - \frac{1}{Z^2} \sum_{\{\tau_i\}=\pm 1} \tau_i\tau_j \mathrm{e}^{\sum_i \beta h_i^z \tau_i + \sum_{\langle i,j\rangle} \beta J_{ij}\tau_i\tau_j} \sum_{\{\tau_i\}=\pm 1} \tau_k \mathrm{e}^{\sum_i \beta h_i^z \tau_i + \sum_{\langle i,j\rangle} \beta J_{ij}\tau_i\tau_j} \\
& - (\langle \tau_i\tau_k \rangle - \langle \tau_i \rangle\langle \tau_k \rangle)\langle \tau_j \rangle - \langle \tau_i \rangle(\langle \tau_j\tau_k \rangle - \langle \tau_j \rangle\langle \tau_k \rangle) \\
=& \langle \tau_i\tau_j\tau_k \rangle - \langle \tau_i\tau_j \rangle\langle \tau_k \rangle - \langle \tau_i\tau_k \rangle\langle \tau_j \rangle - \langle \tau_i \rangle\langle \tau_j\tau_k \rangle + 2\langle \tau_i \rangle\langle \tau_j \rangle\langle \tau_k \rangle.
\end{aligned} \tag{S26}$$

At sufficiently high temperatures, the partition function $Z$ is as follows

$$\begin{aligned}
Z =& \sum_{\{\tau_i\}=\pm 1} \prod_k \mathrm{e}^{\beta h_k^z \tau_k} \prod_{\langle i,j\rangle} \mathrm{e}^{\beta J_{ij}\tau_i\tau_j} \\
=& \prod_{\langle i,j\rangle} \cosh(\beta J_{ij}) \sum_{\{\tau_i\}=\pm 1} \prod_k \mathrm{e}^{\beta h_k^z \tau_k} \prod_{\langle i,j\rangle} [1 + \tau_i\tau_j \tanh(\beta J_{ij})] \\
\sim & \prod_{\langle i,j\rangle} \cosh(\beta J_{ij}) \prod_k 2\cosh(\beta h_k^z)[1 + \sum_{\langle i,j\rangle} \tanh(\beta h_i^z)\tanh(\beta h_j^z)\tanh(\beta J_{ij})].
\end{aligned} \tag{S27}$$

Using this to calculate the free energy, we get

$$\begin{aligned}
F =& -T\sum_{\langle i,j\rangle} \ln[\cosh(\beta J_{ij})] - T\sum_k \ln[2\cosh(\beta h_k^z)] - T\ln[1 + \sum_{\langle i,j\rangle} \tanh(\beta h_i^z)\tanh(\beta h_j^z)\tanh(\beta J_{ij})] \\
\sim & -T\sum_{\langle i,j\rangle} \ln[\cosh(\beta J_{ij})] - T\sum_i \ln[2\cosh(\beta h_i^z)] - T\sum_{\langle i,j\rangle} \tanh(\beta h_i^z)\tanh(\beta h_j^z)\tanh(\beta J_{ij}).
\end{aligned} \tag{S28}$$

In the case of kagomé ice,

$$F = -T[6N\ln[\cosh(\beta J)] + \sum_i \ln[2\cosh(\beta h_i^z)] + \tanh(\beta J)\sum_{\langle i,j\rangle} \tanh(\beta h_i^z)\tanh(\beta h_j^z)]. \tag{S29}$$

Thus, the average value of spins read,

$$\langle \tau_i \rangle = \tanh(\beta h_z)(1 + 4\frac{\tanh(\beta J)}{\cosh^2(\beta h_z)}) \sim \beta h_z(1 + 4\beta J), \tag{S30}$$

$$\langle \tau_i\tau_j \rangle = \tanh^2(\beta h_z)(1 + 4\frac{\tanh(\beta J)}{\cosh^2(\beta h_z)})^2 + \frac{\tanh(\beta J)}{\cosh^4(\beta h_z)} \sim (\beta h_z)^2 + \beta J, \tag{S31}$$

$$\begin{aligned}
\langle \tau_i\tau_j\tau_k \rangle =& \tanh(\beta h_z)^3(1 + 4\frac{\tanh(\beta J)}{\cosh^2(\beta h_z)})^3 + 3\tanh(\beta h_z)(1 + 4\frac{\tanh(\beta J)}{\cosh^2(\beta h_z)})\frac{\tanh(\beta J)}{\cosh^4(\beta h_z)} \\
\sim & (\beta h_z)^3 + 3\beta^2 h_z J.
\end{aligned} \tag{S32}$$

## V. HUSIMI TREE

We calculated the spin correlations using the Husimi tree [1, 2]. The Husimi tree, as shown in Fig. 4(d), is a tree-like structure built with successive generations of triangles. This model is known to be exactly solvable with a recursion

method [3]. The partition function of the Husimi tree of depth $L$ is

$$Z = uZ_{+1,L}^3 + 3Z_{+1,L}^2 Z_{-1,L} + 3dZ_{+1,L}Z_{-1,L}^2 + lZ_{-1,L}^3, \tag{S33}$$

where $u := \mathrm{e}^{\beta(4J+h_z)}, d := \mathrm{e}^{-\beta h_z}, l := \mathrm{e}^{\beta(4J-2h_z)}$, and $Z_{\tau,n}$ is is the partition function at layer $n$ with the value of the terminating spin fixed to $\tau$. To simplify the notation, we define

$$A_n := Z_{+1,n}, \alpha_n := Z_{-1,n}, Y_n := \frac{\alpha_n}{A_n}. \tag{S34}$$

These partition functions obey the following recursion relations:

$$A_n = uA_{n-1}^2 + 2A_{n-1}\alpha_{n-1} + d\alpha_{n-1}^2, \alpha_n = A_{n-1}^2 + 2dA_{n-1}\alpha_{n-1} + l\alpha_{n-1}^2, Y_n = \frac{1 + 2dY_{n-1} + lY_{n-1}^2}{u + 2Y_{n-1} + dY_{n-1}^2}. \tag{S35}$$

When $L \to \infty$, this becomes

$$dY^3 + (2-l)Y^2 + (u-2d)Y - 1 = 0. \tag{S36}$$

By using $Y$, the probability $p_{\tau,\tau'}$ that a spin on the Husimi tree is $\tau$ read

$$p_{+1} = \frac{1}{1+Y^2}, p_{-1} = \frac{Y^2}{1+Y^2}, \tag{S37}$$

and the conditional probability $p_{\tau,\tau'}$ that a neighboring spin is $\tau'$ given that a spin is $\tau$ read

$$p_{+1,+1} = \frac{u+Y}{u+2Y+dY^2}, p_{+1,-1} = \frac{Y+dY^2}{u+2Y+dY^2}, p_{-1,+1} = \frac{1/Y+d}{u+2Y+dY^2}, p_{-1,-1} = \frac{d+lY}{u+2Y+dY^2}. \tag{S38}$$

To simplify the notation, we define

$$P_1 := \frac{1}{1+Y^2}\begin{pmatrix} 1 & Y^2 \\ 1 & Y^2 \end{pmatrix}, P_2 := \frac{1}{u+2Y+dY^2}\begin{pmatrix} u+Y & Y+dY^2 \\ 1/Y+d & d+lY \end{pmatrix}. \tag{S39}$$

Then, the spin correlation of the Husimi tree reads,

$$\langle\tau_i\rangle = \mathrm{tr}[P_1\sigma_z] = -1 + \frac{2}{1+Y^2}, \tag{S40}$$

$$\langle\tau_i\tau_j\rangle_1 = \mathrm{tr}[P_1\sigma_z P_2\sigma_z] = \frac{(u-dY^2) - Y(1-lY^2)}{(1+Y^2)(u+2Y+dY^2)}, \tag{S41}$$

$$\langle\tau_i\tau_j\rangle_2 = \mathrm{tr}[P_1\sigma_z P_2 P_2\sigma_z] = \frac{(u-dY^2)^2 + (1-lY^2)^2}{(1+Y^2)(u+2Y+dY^2)^2}, \tag{S42}$$

$$\chi_A = \frac{u - 3Y + 3dY^2 - lY^3}{u + 3Y + 3dY^2 + lY^3}, \tag{S43}$$

$$\chi_B = \mathrm{tr}[P_1\sigma_z P_2\sigma_z P_2\sigma_z] = \frac{(u-dY^2)^2 - (1-lY^2)^2}{(1+Y^2)(u+2Y+dY^2)^2}, \tag{S44}$$

$$\chi_C = \mathrm{tr}[P_1\sigma_z P_2\sigma_z P_2 P_2\sigma_z] = \frac{(u+Y)(u-dY^2)^2 - (d+lY)(1-lY^2)^2}{(1+Y^2)(u+2Y+dY^2)^3}, \tag{S45}$$

$$\begin{aligned}\chi_D =& \chi_E = \mathrm{tr}[P_1\sigma_z P_2 P_2\sigma_z P_2 P_2\sigma_z] \\ =& \frac{1}{(1+Y^2)(u+2Y+dY^2)^4}[((u+Y)^2 + (1+dY)^2)^2 - Y^2((1+dY)^2 + (d+lY)^2)^2 \\ &+ (u+d+(1+l)Y)^2(1+dY)[-1 + (d-2u)Y + (-1+2l)Y^2 + dY^3]].\end{aligned} \tag{S46}$$

At high temperatures ($T \gg J, h_z$), $u, d, l, Y$ can be expanded as follows:

$$u \sim 1 + \beta(4J+h_z) + \frac{1}{2}\beta^2(4J+h_z)^2 + \frac{1}{6}\beta^3(4J+h_z)^3, \tag{S47}$$

$$d \sim 1 - \beta h_z + \frac{1}{2}\beta^2 h_z^2 - \frac{1}{6}\beta^3 h_z^3, \tag{S48}$$

$$l \sim 1 + 2\beta(2J-h_z) + 2\beta^2(2J-h_z)^2 + \frac{4}{3}\beta^3(2J-h_z)^3, \tag{S49}$$

$$Y \sim 1 - \beta h_z + \beta^2(\frac{1}{2}h_z^2 - 4Jh_z) + \beta^3(-\frac{1}{6}h_z^3 + 4Jh_z^2 - 12J^2h_z). \tag{S50}$$

Then, the spin correlation of the Husimi tree reads,

$$\langle\tau_i\rangle \sim \beta h_z + 4\beta^2 J h_z, \langle\tau_i\tau_j\rangle_1 \sim \beta J + \beta^2(h_z^2 + J^2), \langle\tau_i\tau_j\rangle_2 \sim \beta^2(J^2 + h_z^2) + \beta^3(2J^3 + 8Jh_z^2), \tag{S51}$$

$$\chi_A \sim 3\beta^2 J h_z + \beta^3(h_z^3 + 9J^2 h_z), \chi_B \sim 2\beta^2 J h_z + \beta^3(h_z^3 + 9J^2 h_z), \tag{S52}$$

$$\chi_C \sim \beta^2 J h_z + \beta^3(h_z^3 + 6J^2 h_z), \chi_D = \chi_E \sim \beta^3(h_z^3 + 2J^2 h_z). \tag{S53}$$

This is consistent with the results calculated above using free energy and suggests that $\sigma_{xy}$ in kagomé ice changes sign at high temperatures, reflecting the sign change of chirality. The sign change of chirality is due to the change of spin configuration with increasing temperature. Under high magnetic fields, the ground state is the all-up state, in which all spins on the kagomé lattice point upward, but the population of triangles with two-up-one-down increases as the temperature increases [Fig. 4(e)]. This causes the average value of the chirality to change from positive to negative.

At low magnetic field ($T \gg h_z$), $u, d, l, Y$ can be expanded as follows:

$$u \sim (1 + \beta h_z)j, d \sim 1 - \beta h_z, l \sim (1 - 2\beta h_z)j, Y \sim 1 + \frac{3j+1}{j-5}\beta h_z, \tag{S54}$$

where $j = \mathrm{e}^{4\beta J}$. Then, the spin correlation of the Husimi tree reads,

$$\langle\tau_i\rangle \sim \frac{1+3j}{5-j}\beta h_z, \langle\tau_i\tau_j\rangle_1 \sim -\frac{1-j}{3+j}, \langle\tau_i\tau_j\rangle_2 \sim (\frac{1-j}{3+j})^2, \tag{S55}$$

$$\chi_A \sim -3\frac{1-j}{5-j}\beta h_z, \chi_B \sim -\frac{(1-j)(7+j)(1+3j)}{(3+j)^2(5-j)}\beta h_z \tag{S56}$$

$$\chi_C \sim -\frac{(1-j)(1+3j)(5+10j+j^2)}{(3+j)^3(5-j)}\beta h_z, \chi_D = \chi_E \sim \frac{(1-j)^2(1+3j)(17+14j+j^2)}{(3+j)^4}\beta h_z \tag{S57}$$

At low temperatures ($T \ll J$), $Y$ can be approximated as follows:

$$Y = \frac{1}{\sqrt{2}} - \frac{u}{4} + \frac{3}{8}d + \frac{l}{4\sqrt{2}}. \tag{S58}$$

Then, the spin correlation of the Husimi tree reads,

$$\langle\tau_i\rangle \sim \frac{1}{3} + \frac{2\sqrt{2}}{9}u - \frac{\sqrt{2}}{3}d - \frac{2}{9}l, \langle\tau_i\tau_j\rangle_1 \sim -\frac{1}{3} + \frac{4\sqrt{2}}{9}u + \frac{2}{9}l, \langle\tau_i\tau_j\rangle_2 \sim \frac{1}{3} - \frac{\sqrt{2}}{9}u - \frac{d}{\sqrt{2}} - \frac{5}{9}l. \tag{S59}$$

[1] K. Husimi, J. Chem. Phys. **18**, 682 (1950).
[2] F. Harary and G. E. Uhlenbeck, Proc. Natl. Acad. Sci. **39**, 315 (1953).
[3] M. Potts and O. Benton, Phys. Rev. B **106**, 054437 (2022).
